# Supplementary material for: YouTube Recommendations Reinforce Negative Emotions: Auditing Algorithmic Bias with Emotionally-Agentic Sock Puppets
Source: arXiv:2501.15048 source file (2025-01-25)
Supplement: Supplementary file 1 [file 9.appendix.tex]

\section{Appendix}

\subsection{Methods and Validations}

\para{InnerTube and YouTube}
\para{Making the embeddings.}
